# Supplementary material for: Polymer translocation under a pulling force: scaling arguments and threshold forces
Source: arXiv:1711.10832 ancillary file (2017-11-29)
Supplement: Supplementary file 1 [file supplemental-material-polymer.pdf]

# Supplemental Material for: Polymer translocation under a pulling force: scaling arguments and threshold forces


Timothée Menais

*CEA, CNRS, Univ. Grenoble Alpes, INAC-SyMMES, F-38000 Grenoble, France*

*UOIT CNABLAB, Oshawa, ON L1H 7K4, Canada*



(Dated: November 28, 2017)



This document gathers all the Electronic Supplementary Informations concerning the paper entitled: "Polymer translocation under a pulling force: scaling arguments and threshold forces"


## I. SCALING EXPONENTS FOR POLYMERS IN SOLUTION

Before starting any work on translocation issues, we first validate our polymer model in solution by investigating static properties of three different polymer models : an ideal linear polymer without excluded volume interactions (theoretically defined by a random walk), a linear polymer with excluded volume effects (defined by a self avoiding walk or SAW) and a structured polymer with excluded volume effects and adjacent bases attached to the backbone.

The static properties studied are the mean end-to-end distance and the gyration radius in blue for the ideal polymer, in green for the linear SAW polymer and in red for the structured SAW polymer (See figure 1). For our ideal polymer, we indeed find results close to the behaviour of a gaussian chain with the polymer size scaling like $N^\nu$ with $\nu = 0.53$ and 0.51 for the end-to-end distance and the giration radius respectively instead of the expected $\nu = 1/2$ exponent. For both polymer models presenting excluded volume effects, we found results close to the expected Flory exponent $\nu \simeq 0.588$. For the linear SAW polymer the exponents of $\nu = 0.58$ and 0.64 for the end-to-end distance and the gyration radius have been obtained. For the structured SAW polymer, larger values have been observed ($\nu = 0.71$ and 0.70 respectively). The scaling exponents are often overestimated due to finite size effects. In case of the structured polymer, the side chains composed of the bases tends to increase the effective persistent length due to the extra excluded volume interactions. Thus, this may explain the larger effective exponent $\nu \simeq 0.7$ observed.

After the static properties, we also investigated dynamical properties and found a nearly inverse linear scaling for the diffusion coefficient of the structured polymer ($D \sim N^{-1.04}$) and a linear scaling for the bulk friction coefficient ($N^{1.03}$) as theoretically expected (see figure 2). Furthermore, the product of both the diffusion and the bulk friction is close to the impose temperature verifying the Einstein's relation.

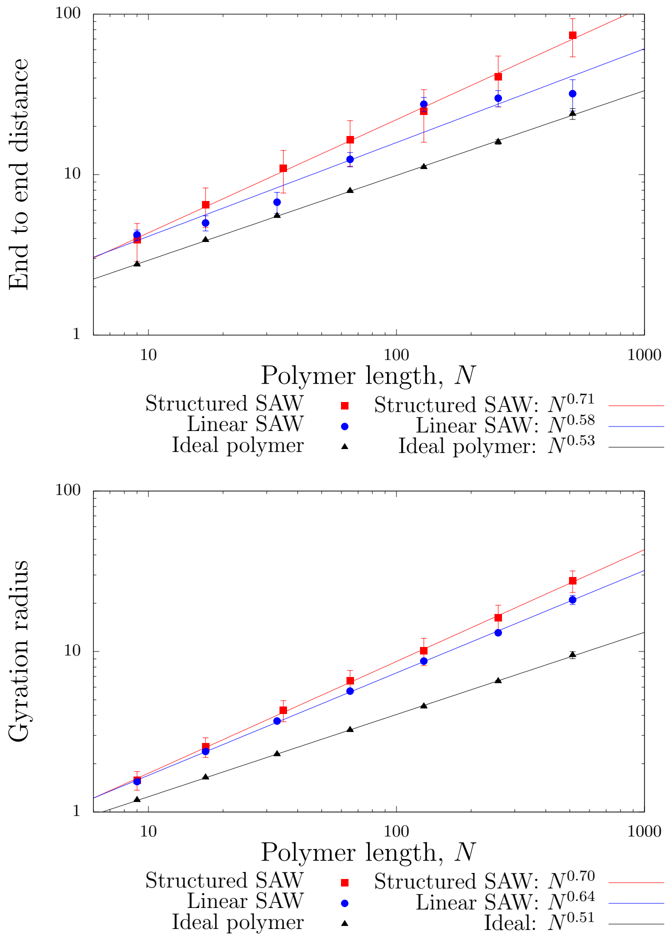


FIG. 1. Evolution of the mean end-to-end distance (top) and gyration radius (bottom) with the polymer chain length for an ideal linear polymer (blue), a linear self avoiding polymer (green) and our structured self avoiding polymer (red).

## II. LARGE FORCE TRANSLOCATION SCALINGS

The translocation time $\tau \sim 1/F^\delta$ depends on the force exerted on the trnaslocating polymer with a scaling exponent $\delta = 1$ generally expected. However, at large forces, lower values of the exponent are generally observed numerically. In order to understand this decrease of the

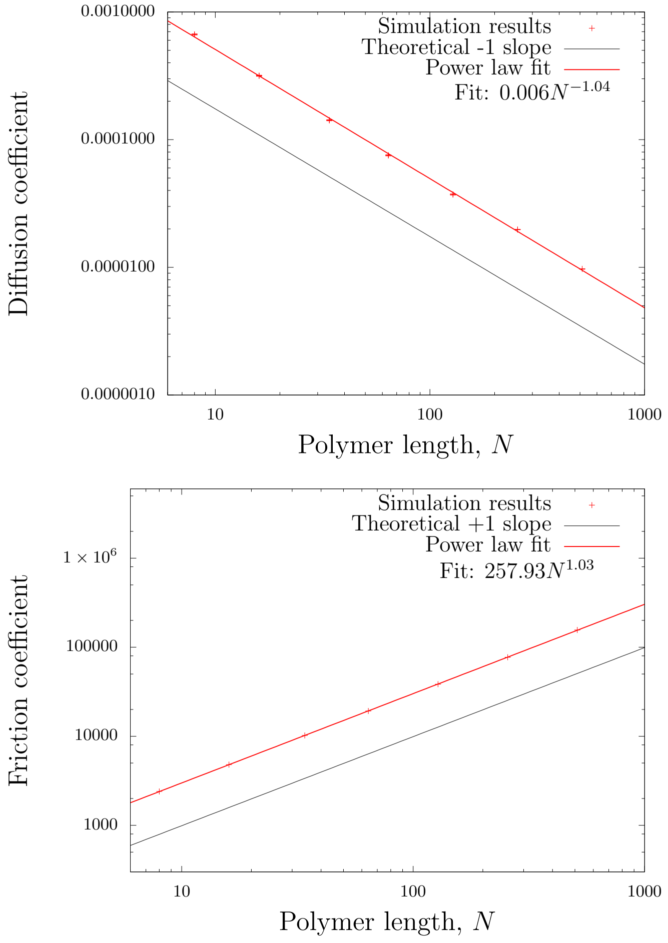


FIG. 2. Evolution of the diffusion coefficient (top) and the friction coefficient (bottom) with our structured polymer chain length. Accordingly with polymer theory, the diffusion coefficient scales as $1/N$ and the friction coefficient as $N$.

critical exponent $\delta$ at large forces, we simulated deterministic polymers. Namely, a linear self avoiding polymer (with $N = 16$ beads) is placed with the first grain centered within the pore. The chain is then placed at rest on a line orthogonal to the membrane. No temperature is imposed to the polymer leading to the deterministic simulation (no noise is present during the simulation). The polymer pulling is imposed at various forces $F$, bond strengths $k$ and friction parameters $\nu$. Table I presents the scaling exponents $\delta$ estimated for the large forces regime ($F > 20$). For low solvent friction and high bond strengths, $\delta \approx 1$ is recovered as expected. However, for high friction and/or low bond strength, the estimated scaling exponent $\delta$ decreases.

Our interpretation is that in most simulations, included those performed with a bias force within the pore (forces from electrophoretic interactions for example) $\nu$ and $k$ values are not well chosen giving bonds whose extension are not negligible at high forces. Thus, the decrease of the scaling exponent $\delta < 1$ is directly related to this bond extension and not as proposed previously due to excluded volume effects in the trans side due to overcrowding of the polymer beads at the exit of the pore [1]. Indeed, this over-crowding is completely lacking in our simulations where the polymer is pulled by one end and is thus in an extended form in the trans side.

| $\nu$ value | $k$ value | $\delta$ estimation |
|---|---|---|
| 0.1 | 30 | 0.989 ± 0.007 |
| 0.33 | _ | 0.972 ± 0.004 |
| 1 | _ | 0.884 ± 0.05 |
| 3 | _ | 0.62 ± 0.02 |
| 10 | _ | 0.51 ± 0.02 |
| 30 | _ | 0.478 ± 0.02 |
| 1 | 3 | 0.85 ± 0.02 |
| 1 | 300 | 0.90 ± 0.02 |

TABLE I. High forces range estimations of $\delta$ for several bond strength ($k$) and grain/solvent friction coefficients ($\nu$).

## III. DISTRIBUTION OF TRANSLOCATION TIMES

We analysed our translocation times distribution with a first passage probability density function suggested by Ling and Ling for an electrophoretic bias [2]:

$$F_1(t) = \frac{L}{\sqrt{4\pi D t^3}} e^{-(L-vt)^2/4Dt} \quad (1)$$

with $L$ being the length of the polymer chain, $D$ the diffusion coefficient of the membrane along the polymer and $v$ the mean translocation velocity. The distribution is fitted using only two parameters, $x$ and $y$:

$$F_1(t) = \frac{1}{\sqrt{\pi t^3}} x e^{-(1-yt))^2 x^2/t} \quad (2)$$

with $x = L/\sqrt{4D}$ and $y = v/L$.

Being in a reasonable force range and using a bond length of 1, we can replace the chain length $L$ directly by the number of monomers $N$. The translocation times distributions were fitted against equation 2 with the GNUPLOT software (see figure 3). We obtained very good results for the parameter $y$. The mean translocation velocity obtained is identical to the one we get simply by dividing the mean translocation time by the chain length. Concerning the parameter $x$ however, a large range of acceptable values as fitting parameters prevents us from determining a reliable diffusion coefficient of the membrane along the polymer (as the model proposed in [2] is in the referential of the polymer chain). Similar distributions are obtained by de Haan et al. [3] in the case of pulling forces but were not interpreted as first passage probability density.

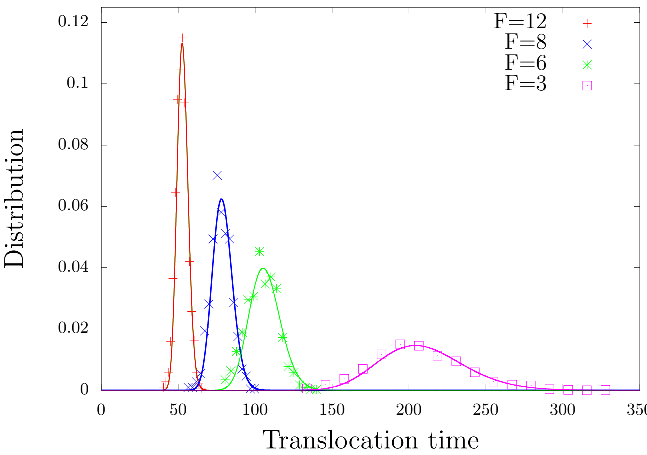


FIG. 3. Translocation time distributions for our simple linear polymer (pulled at forces F=3, 6, 8 and 12) and their fit with a first passage probability density function.

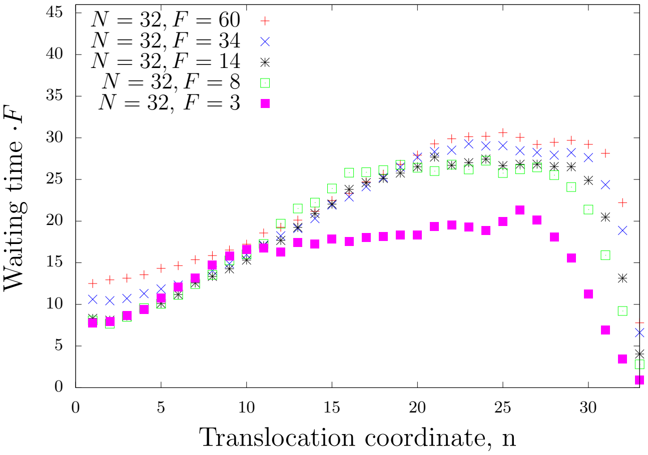


FIG. 4. Rescaled waiting time ($w^* = wF$) as function of the translocation coordinate $n$ for a given polymerisation index ($N = 32$). The rescaling is perfect up to medium forces ($F < 20$). Then bonds extensibility modifies the $1/F$ rescaling.

In our investigation of the translocation velocity we used the value obtained by dividing the mean translocation time by the chain length as it is the proper definition of the mean translocation velocity and easier to calculate.

## IV. SCALING ANALYSIS FROM THE WAITING TIMES DISTRIBUTION

In this study, we analyzed the waiting time as function of the translocation coordinate for a given pulling force $F$ and several polymerisation indexes $N$. Here, we plot a first rescaling of the waiting time (the waiting time multiplied by the applied force $F$) in function of

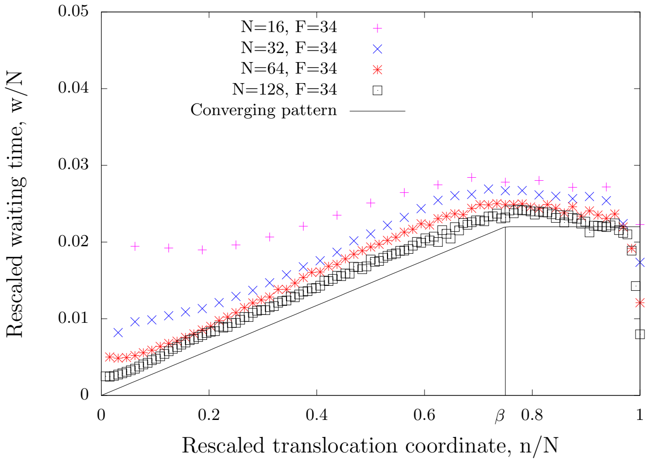


FIG. 5. Rescaled waiting time ($w^{**} = w/N$) as function of the rescaled translocation coordinate $n^* = n/N$ for a given polymerisation index ($N = 32$). The rescaling is pgetting better with increasing $N$ as finite size effects vanish and the value of the variation of the predicted value $\beta$ diminishes. the $1/F$ rescaling.

the translocation coordinate for a polymerisation index $N = 32$ on figure 4. The curves rescale correctly at the origin and for the initial slope of translocation coordinates, except for the large forces ($F = 34$ and $F = 60$) due to the bond extension described in the previous section and at low forces $F = 3$ for the plateau. In this later case, the value of $\beta$ is lower as the pulling force is lower and diffusion occurs earlier. This rescaling indicates that $w(n) = a(F)+b(F)n$ with $a(F) = a'/F$ and $b(F) = b'/F$ for the initial regime dominated by the force.

We also provide a second rescaling (the waiting time divided by the polymer length $N$ in function of the translocation coordinate also divided by the chain length for a pulling force $F = 34$) on figure 5. This rescaling shows that with increasing $N$, finite size effects become less relevant while the value of $\beta$ doesn't vary much in the case of a high pulling force.

We have also estimated the fraction of the polymer ($\beta = n^*/N$) for which the change from force driven regime linear behavior to diffuse plateau regime for the waiting time. We adjusted the equation described in the paper with the full length of the polymer $N$ (without correction) and with an effective length $N_e = N - 4$ to take into account the tail retraction (with length correction). The results are plotted on figure 6 and enable us to estimate the prefactor $C = 4.89$ defined in the paper.

In equation 13 of the main paper we have shown that there is a prefactor before the $\tau \propto N^2/F$ term that remains constant for $A = 2CN/F^2 < 1$, this prefactor is plotted on figure 7.

On figure 8 we have plotted the average waiting time obtained for our three polymer models for a higher pulling force ($F = 34$). As expected, the structure-

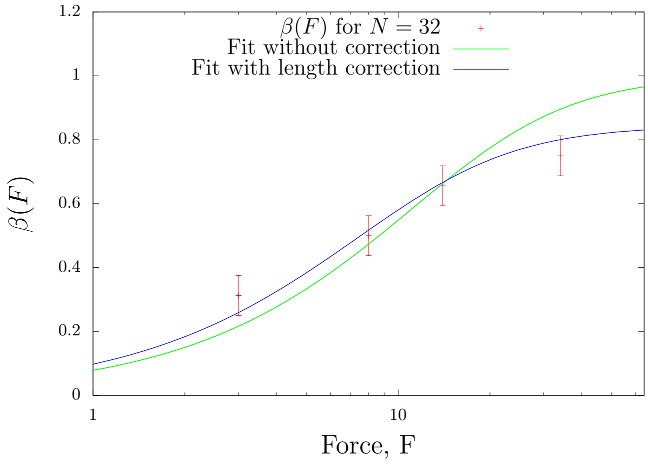


FIG. 6. Fraction of polymer coordinate $\beta(F,N) = n^*/N$ corresponding to the crossover between force driven regime and unbiased regime as function of the pulling force $F$ for a given polymerisation index $N = 32$. The formula given in the main paper fits correctly our results with a length correction taking the tail retraction into account. This fit enables us to estimate the prefactor $C = 4.89$.

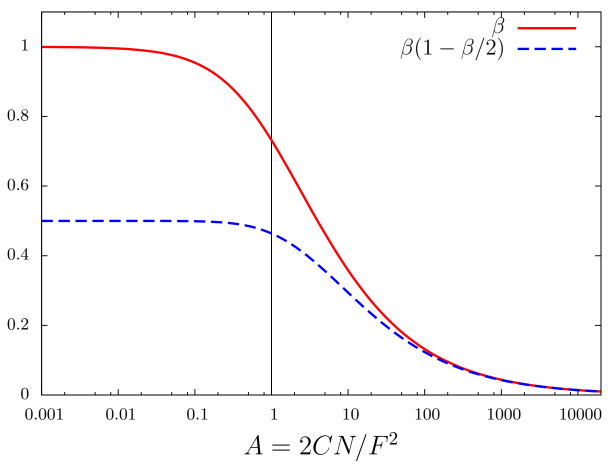


FIG. 7. Fraction of regime change ($\beta$ in red plain line) and pre-factor in eq.13 (blue dotted line) plotted in function of $A = 2CN/F^2$.

pore interactions are less important than for lower pulling forces as observed on figure 10 of the main paper.

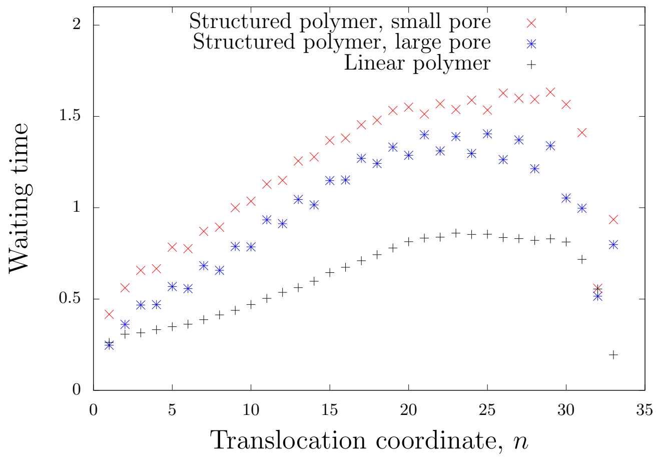


FIG. 8. Average waiting time depending on the translocation coordinate at given high force ($F = 34$) and polymer chain length ($N = 32$) for our linear polymer (black) and our structured polymer in the case of a large (blue) and small (red) pore.


[1] V. V. Palyulin, T. Ala-Nissila, and R. Metzler, Soft Matter **10**, 9016 (2014).

[2] D. Y. Ling and X. S. Ling, Journal of Physics: Condensed Matter **25**, 375102 (2013).

[3] H. W. de Haan, D. Sean, and G. W. Slater, Physical Review E **91** (2015), 10.1103/physreve.91.022601.
